# Supplementary material for: Object Detection with a Unified Label Space from Multiple Datasets
Source: arXiv:2008.06614 source file (2020-08-15)
Supplement: Supplementary file 1 [file appendix.tex]

\section{Discussion points from group meeting \& action items}

\begin{itemize}
\item We make the argument that gradients from more datasets help in improving our results. This should be justified with an experiment where we sequentially add new datasets. Problem with this is that results will be highly dependent on the order in which we present the datasets.
\item We need to justify our choice of datasets.
\item UOD setting: Need to think more about this, but essentially one thing we can try to show is that it does not hurt our method if you through in a set of unrelated datasets. Can we do this on the 11 datasets from UOD?
\item Add literature on weakly supervised object detection in the related work section
\item Our approach can be seen as a generalization of fine-tuning without catastrophic forgetting mechanisms. Can we do experiments that compare with such mechanisms? We could train a model on dataset A, then fine-tune on dataset B with a mechanism to avoid catastrophic forgetting. Then we measure performance. Obviously, this approach already has disadvantages by design: the training process is sequential and the order the datasets are presented will matter.
\item To measure the domain gap between two datasets or two images or even two bounding boxes, we could use MMD (maximum mean discrepancy). If we have a reliable measure, we can try to integrate this into the pseudo labeling losses.
\item How do we deal with annotation inconsistencies? Two prominent examples are: amodal vs. only-visible-part annotation for human bodies or the tightness of face annotations. \todo{This is an important issue we need to address!}
\item Implement baselines with partial labelling losses
\item Another motivating example for our paper could be the following: A typical machine learning (deployment) pipeline, consists of a few steps that repeat: Collect and annotate data, train a model, evaluate the model, analyze its errors and collect new data and annotations similar to the error cases, which hopefully alleviates open problems. Now, a typical situation when analyzing errors is that only a few categories under-perform whereas other categories already reached a satisfactory level of performance.  However, after we have collected data specific to the error cases, we still need to annotate ALL categories, even the ones that already achieve good performance in order to not jeopardize those categories. With our approach on the other hand, we can afford to only annotate a few categories for the newly collected data and let the algorithm know that for this new data annotations for some categories are missing.
\item \todo{We to need think about splitting the test/val sets sensibly to have a small part left for potentially training an unsupervised domain adaptation method.}
\item \todo{When doing a domain \emph{generalization} experiment, we should have the validation set in the domain of the training images, but only the test set on the new domain.  This is an additional challenge for us in terms of dataset splits and annotation collection, I think.}
\item Can we have one experiment where we directly compare with Wang~\etal~\cite{Wang_2019_CVPR}? Maybe, we do not need to add the datasets that are completely out-of-domain because this would be unfair. They essentially have a Person-Cartoon and a Person-Real detector. I guess for our work to compete here, we would also need sub-categories for these types.  I would give this point low priority, it's just here to satisfy the ``lazy reviewer''.
\item We should also think about what happens if we would replace the softmax with a per-category sigmoid as in RetinaNet. If our initial thoughts are conclusive, we should argue here why it does not make a difference if you use sigmoid or softmax.
\item \todo{Oh~\etal~\cite{Oh_2015_ICCV} investigate full human analysis and also work with \pipa~\cite{Zhang_2015_CVPR} but do not provide additional annotations, only a new train/test split (\url{https://www.mpi-inf.mpg.de/departments/computer-vision-and-machine-learning/research/people-detection-pose-estimation-and-tracking/person-recognition-in-personal-photo-collections/}).  We should look into this paper but we probably need to annotate faces in \pipa.}
\end{itemize}

%%% Local Variables:
%%% mode: latex
%%% TeX-master: "../uod_with_pseudolabeling"
%%% End:
